# Supplementary material for: Two-Dimensional hybrid perovskites sustaining strong polariton interactions at room temperature
Source: arXiv:1811.04041 ancillary file (2018-11-09)
Supplement: Supplementary file 1 [file Supplementary_Info.pdf]

# Two-Dimensional hybrid perovskites sustaining strong polariton interactions at room temperature

A. Fieramosca[1,2*], L. Polimeno[1,2,4*], V. Ardizzone[1,2†], L. De Marco[1,‡], M. Pugliese[1], V. Maiorano[1], M. De Giorgi[1], L. Dominici[1], G. Gigli[1,2], D. Gerace[3,1], D. Ballarini[1], D. Sanvitto[1,4].

[1]*CNR Nanotec, Institute of Nanotechnology, via Monteroni, 73100 Lecce, Italy.*

[2]*Dipartimento di Matematica e Fisica, Università del Salento, via Arnesano, 73100 Lecce, Italy.*

[3]*Dipartimento di Fisica, Università degli Studi di Pavia, via Bassi 6, 27100 Pavia, Italy. and*

[4]*INFN Istituto Nazionale di Fisica Nucleare, Sezione di Lecce, 73100 Lecce, Italy.*

* These autors equally contributed to this work

† Electronic Address: v.ardizzone85@gmail.com

‡ Electronic Address: luisa.demarco@nanotec.cnr.it

# Supplementary Information

## I. MATERIAL SYNTHESIS

- **Chemicals and Reagents**: Phenethylammonium iodide ($\geq$ 99%) was purchased from Greatcell Solar. Lead(II) iodide ($PbI_2$) ($\geq$ 99%), hydriodic acid (HI) ($\geq$ 57 wt%), dichloromethane, gammabutyrolactone were purchased from Sigma Aldrich. All chemicals were used as received without any further purification.

- **Synthesis of 2D perovskite**: 498 mg phenethylammonium iodide and 461 mg $PbI_2$ were dissolved in 1 mL gammabutyrolactone and stirred at 70°C for 1 hour. 2D perovskite single crystals were prepared by Anti-solvent Vapor assisted Crystallization method [1] and subsequent mechanical exfoliation as follows: 200 $\mu$m thick glass was cleaned with acetone and water in ultrasonic bath for 10 min each. Then it was soaked into a washing solution ($H_2O_2/NH_3/H_2O$ 5:1:1, v/v) and heated at 80°C for 10 min to remove organic contamination and finally rinsed 10 times in water. 5 $\mu$L of the perovskite solution is deposited on one of the substrate and immediately after capped by the second glass substrate. Then, 2 mL of DCM in a small Teflon beaker is placed at the top of the substrates. Substrates and beaker are placed in a bigger screw-capped Teflon container and left undisturbed overnight. Millimetre-sized crystals formed in between the two substrates were exfoliated with SPV 224PR-M Nitto Tape in order to obtain the desired thickness.

## II. MICROCAVITY FABRICATION

A 170 $\mu$m cover slip (Carlo Erba) has been used as a substrate. The glass surface was cleaned with acetone, iso-propyl alcohol and deionized water (DI) in an ultrasonic bath, then dried with high-purity $N_2$ gas. To fabricate highly reflective DBRs, seven pairs of $TiO_2/SiO_2$ (61 nm/100 nm) multilayers were deposited by radio-frequency (RF) sputtering process in an Argon atmosphere under a total pressure of $6{\cdot}10^{-3}$ mbar and an RF power of 250 W. During the deposition the substrates were warmed at 250 °C. Perovskite crystals are grown overnight after the deposition of the first DBR. Subsequently, seven other pairs of $SiO_2/TiO_2$

(103 nm/63 nm) were deposited under the same conditions to close the microcavity, except for the substrate's temperature that is kept at 50 °C to avoid damaging of the crystals. Optical constants (n and k) of DBR's materials were separately measured via ellipsometric measurements (J.A. Wollam-EC-400) for both temperatures of deposition.

## III. ABSORPTION AND PHOTOLUMINESCENCE

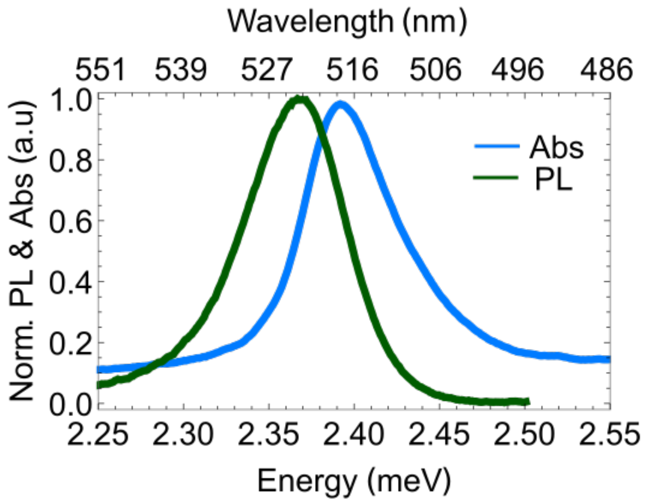


Figure 1: Absorption (Blue) and photoluminescence (Green) spectra measured on top of a PEAI single crystal with a 488nm CW laser.

## IV. OPTICAL SETUP

- **Microcavity measurements**: In Fig.S2 is reported a sketch of the experimental configuration used to measure the microcavity sample (Fig.4). A 50 fs pulsed laser (Coherent, TOPAS-Prime 10 kHz, FWHM=22 meV) resonantly excites polaritons at k=0 through a 10X objective (Rolyn-Rau, N.A.=0.3) in a transmission configuration. A 20X objective (Zeiss, N.A.=0.8) is used to detect the signal and a lenses system allow us to simultaneously detect the real space and the back focal plane. A 300 mm spectrometer (Princeton Instruments, Acton Spectra Pro SP-2300) coupled to a charge coupled device (Princeton Instruments, Pixies 400) is used to analyze the signal. The polarization of the excitation laser is controlled by using a quarter-wave plate (AQWP05M-600) along the excitation line. For photoluminescence measurements (Fig.4a) a CW laser

488 nm is used to excite the perovskite crystal and a 500 nm cut-off filter (Thorlabs-FEL0500) is used to filter the laser.

- **Slab measurements**: For measurements reported in Fig.2 and Fig.3 a 60X oil immersion microscope objective (Olympus, N.A.=1.49) is used to excite the system in a reflection configuration [2]. Blueshift measurements are performed by using the same pulsed laser mentioned above while for reflectivity maps a Xenon light source (Korea Spectral Products-ASB-XE-175) is used.

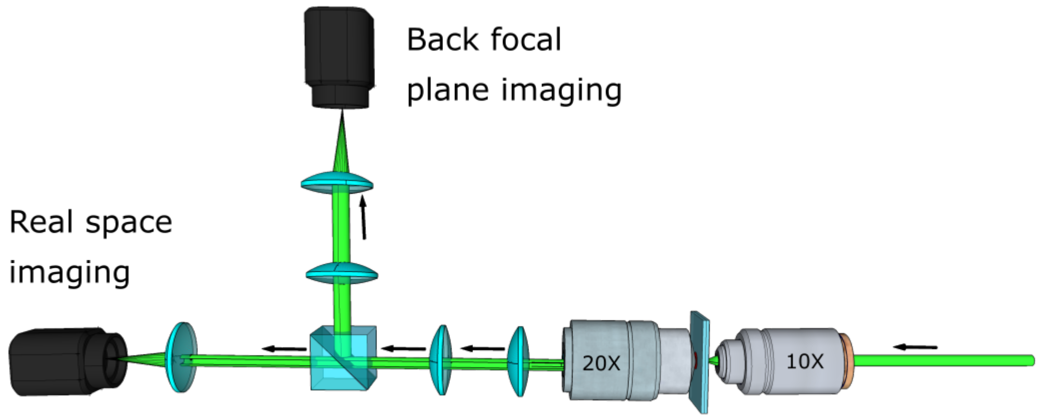


Figure 2: Optical setup used to measure the microcavity sample. A pulsed laser (50 fs, 10kHz, FWHM=22meV) resonantly excites polaritons with zero momentum into the system with a controlled polarization. Along the detection line a lenses system allow the simultaneous detection of back focal plane and real space

## V. INTERACTION CONSTANT

- **Slab:** With reference to the data shown Fig.4, we calculate the incident pulse energy $E_{tot} = \frac{P}{R}$, where P is the incident power and $R = 10$ kHz is the repetition rate, with an excitation spot area of S=20 $\mu$m$^2$. In order to calculate the absorbed energy, and than the polariton density $n_{pol}$, we make a conservative approximation considering that the total injected energy is completely absorbed. From reflectance profiles we can

assume that 60% of the incident energy is reflected and 40% is injected into the system, neglecting the transmission thanks to TIR configuration (see the spectral modulation of excitation laser envelope caused by polariton modes, Fig.4c). Doing so, we consider that the absorbed energy is 40% of $E_{tot}$. With this assumptions we estimated $n_{pol}$ and exciton density $n_{exc}$, as follow:

$$n_{pol} = 0.4 \cdot \frac{E_{tot}}{e_p \cdot S} \tag{1}$$

$$n_{exc} = n_{pol} \cdot X \tag{2}$$

where $e_p$ is the polariton energy, X is the excitonic component (X=$|\chi_{LP}|^2$, $\chi_{LP}$ is the excitonic Hopfield Coefficient). Assuming the electromagnetic field is spread over the whole crystal thickness (Thickness = 5 $\mu$m, LayerNumber = 3000) we calculated the exciton density per layer (where layer thickness represents the sum of inorganic and organic part) dividing the total exciton density for the number of layer. Considering the following relation:

$$\Delta E_{exc} = \frac{\Delta E_{pol}}{X} = g_{exc} \cdot n_{exc/layer} \tag{3}$$

where $\Delta E_{exc}$ is the exciton blueshift, $\Delta E_{pol}$ is the polariton blueshift and $g_{exc}$ the exciton-exciton interaction constant, we are able to link our experimental data, taken at different detunings, to the exciton properties. Figure S3 shows that by plotting $\frac{\Delta E_{pol}}{X}$ as a function of $n_{exc/layer}$ the experimental data are fittable with the same slope for both detunings, represented by red and blue points. From a linear fit of the data we found a value of $g_{exc,lay} \geq 1 \pm 0.2$ $\mu$eV$\cdot\mu$m$^2$ [3].

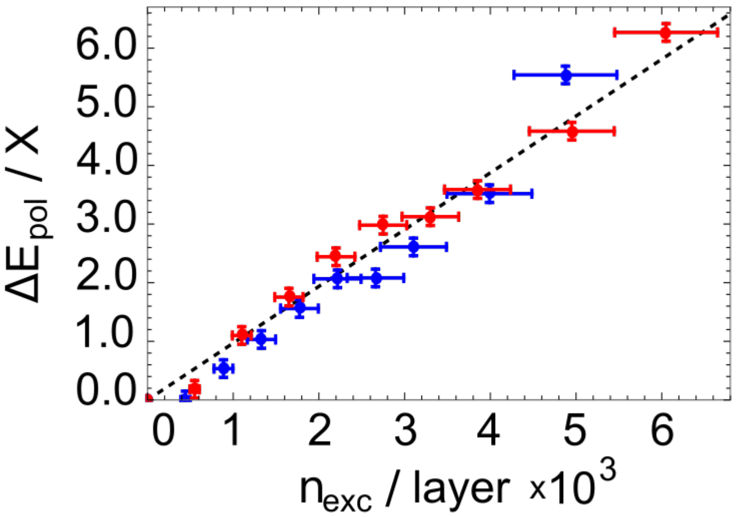


Figure 3: Exciton blueshift as a function of exciton density per QW. Blue and red dots are relative to two different detunings, shown in Fig.4. $g_{exc,lay} \geq 1\pm0.2$ $\mu$eV$\cdot\mu$m$^2$ is the slope of a linear fit of the data (Black Dashed).

- **Microcavity:** The estimation of exciton interaction constant has been done considering a linearly polarised pulsed laser exciting at k=0 the microcavity sample. Following the procedure described above we calculated the exciton blueshift as a function of the exciton density per layer. For this measurement we are considering that the total injected power is half of total incident power, neglecting scattering losses and considering that total injected power is completely absorbed by the system. The crystal has a thickness of 170 nm (Fig. S4a) measured via profilometer before the growth of second Bragg mirror. The corresponding data are shown in Fig. S4b. In order to estimate the interaction constant we are taking into account the range where the blueshift is linear [4] as a function of exciton density per layer. By using a linear fit of the data we obtain a value of the slope of figure 4b $g_L \simeq 1.5\pm0.5$ $\mu$eV$\cdot\mu$m$^2$. Considering the spin dependent interaction (Fig. 2 of the main text), the value of exciton interaction constant is $g_{exc,lay} \simeq 3\pm0.5$ $\mu$eV$\cdot\mu$m$^2$.

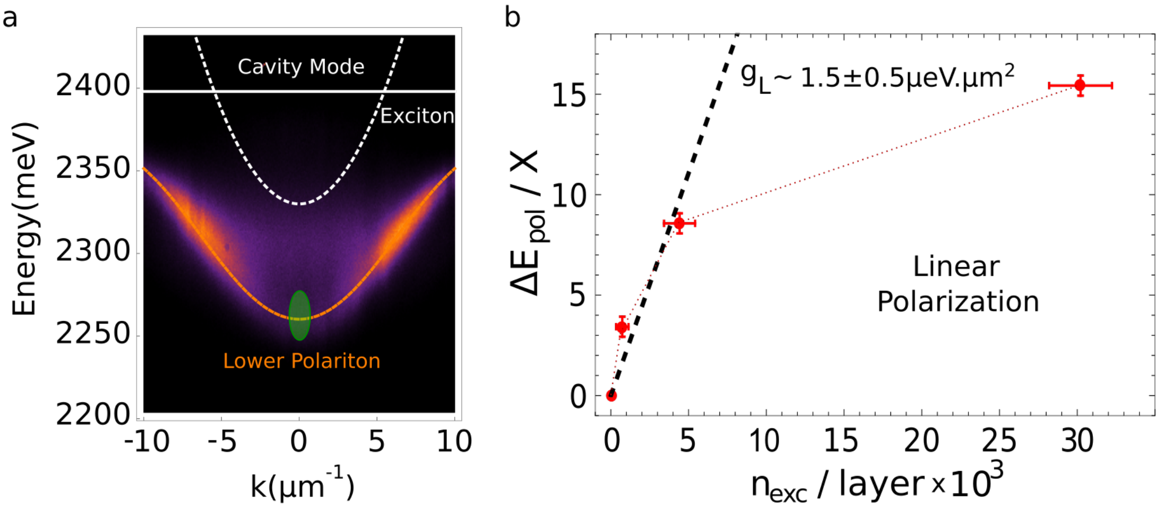


Figure 4: a) Energy vs in plane momentum photoluminescence map of a 170 nm single perovskite crystal embedded in the microcavity. $\hbar\Omega = 170meV$, $E_C = 2.325eV$, $E_X = 2.4eV$. The exciton fraction at k=0 is 0.35. b) Exciton blueshift as a function of exciton density per QW, considering a linearly polarized pulses laser excitation. $g_L \simeq$ 1.5±0.5 $\mu$eV·$\mu$m$^2$ is the slope of a linear fit of the data (Black Dashed).

[1] F. Lédée, G. Trippé-Allard, H. Diab, P. Audebert, D. Garrot, J.S. Lauret, and E. Deleporte. *CrystEngComm*, 19–2598-2602, Mar 2017

[2] A. Fieramosca, L. De Marco, M. Passoni, L. Polimeno, A. Rizzo, B. L. T. Rosa, G. Cruciani, L. Dominici, M. De Giorgi, G. Gigli, L. C. Andreani, D. Gerace, D. Ballarini, and D. Sanvitto. Tunable out-of-plane excitons in 2d single-crystal perovskites. *ACS Photonics*, 5:41794185, Sep 2018.

[3] K. S. Daskalakis, S. A. Maier, R. Murray, and S. Kéna-Cohen. Nonlinear interactions in an organic polariton condensate. *Nature Materials*, 13(3):271278, Feb 2014.

[4] F. Barachati, A. Fieramosca, S. Hafezian, Jie Gu, B. Chakraborty, D. Ballarini, L. Martinu, V. Menon, D. Sanvitto, and S. Kéna-Cohen. Interacting polariton fluids in a monolayer of tungsten disulde. *Nature Nanotechnology*, 13(5):906909, May 2018.
